# Supplementary material for: Charge-Density Wave Driven Giant Thermionic-Current Switching in 1T-TaS$_{2}$/2H-TaSe$_{2}$/2H-MoS$_{2}$ Heterostructure
Source: arXiv:2209.02024 source file (2022-09-05)
Supplement: Supplementary file 1 [file supporting_info.pdf]

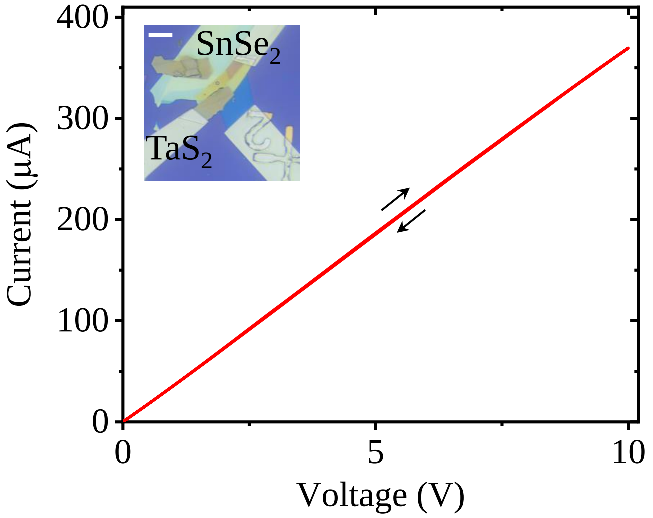


Figure 1: I-V characteristics of $TaS_2/SnSe_2$ junction at room temperature. The inset shows the optical image of the device. Scale bar: 10 $\mu m$. Forward and reverse sweeps are indicated by black arrows.

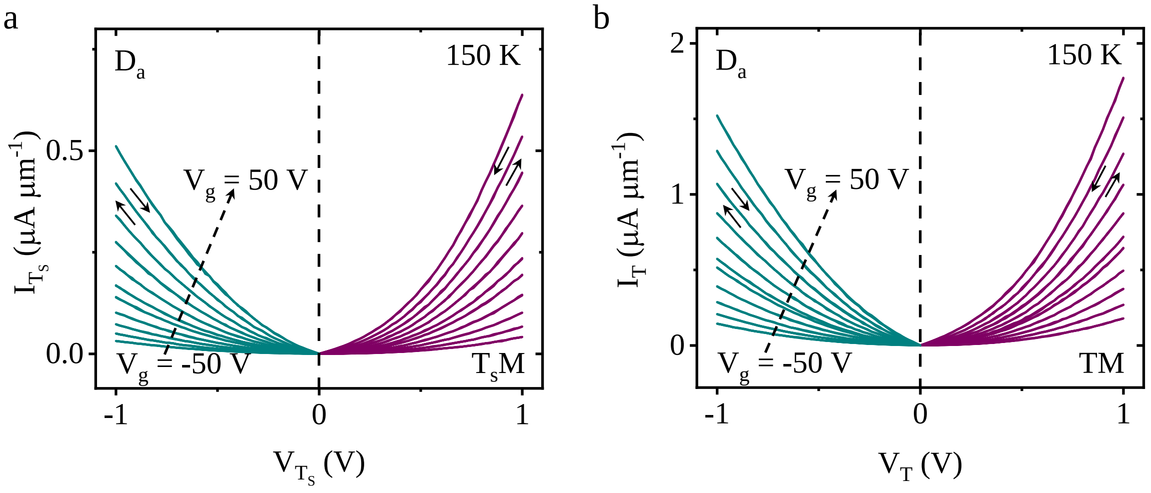


Figure 2: **Electrical characterization of triple layered device $D_a$.** (a),(b) I-V characteristics of $TaSe_2/MoS_2$ junction (probed between terminals $T_S$ and M keeping terminal T open) [in (a)] and $TaS_2/MoS_2$ junction (probed between terminals T and M keeping terminal $T_S$ open) [in (b)] for $V_g$ varying from −50 V to 50 V in steps of 10 V at 150 K. Forward and reverse sweeps are indicated by black arrows.

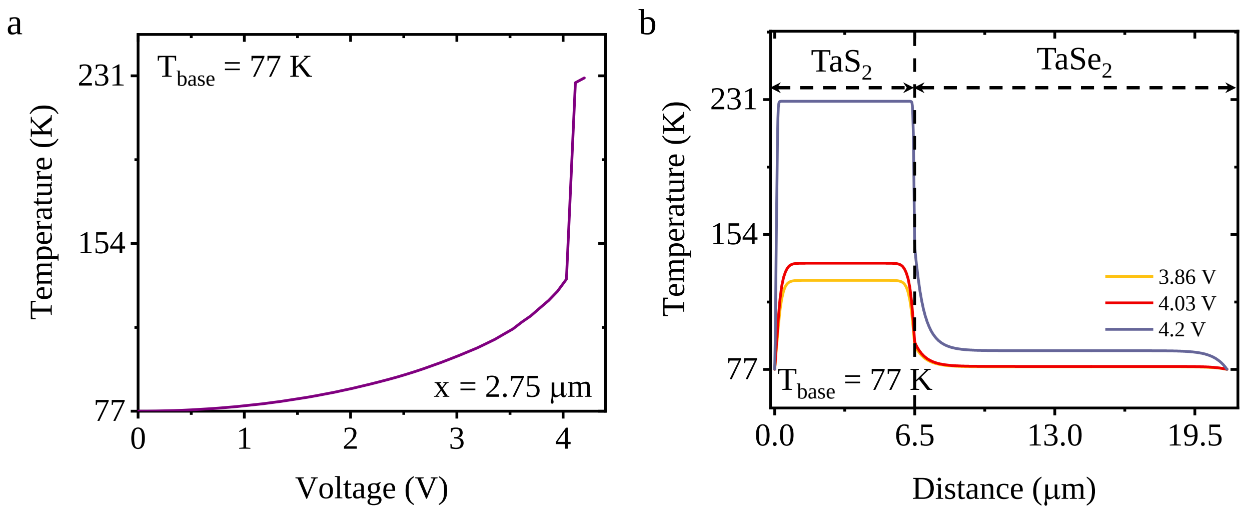


Figure 3: **Simulated temperature profile along $TaS_2/TaSe_2$ channel.** (a) Temperature profile simulated at the middle of the $TaS_2$ channel of device $D_b$ as the function of voltage for base temperature ($T_{base}$) of 77 K. (b) Simulated temperature variation along the $TaS_2/TaSe_2$ channel at bias voltage of 3.86 V (before transition), 4.03 V (at transition) and 4.2 V (after transition) for $T_{base}$ of 77 K. Note that the thickness of the $MoS_2$ and $TaSe_2$ layers being few nanometers, all the materials in the triple junction experience a large change in temperature.

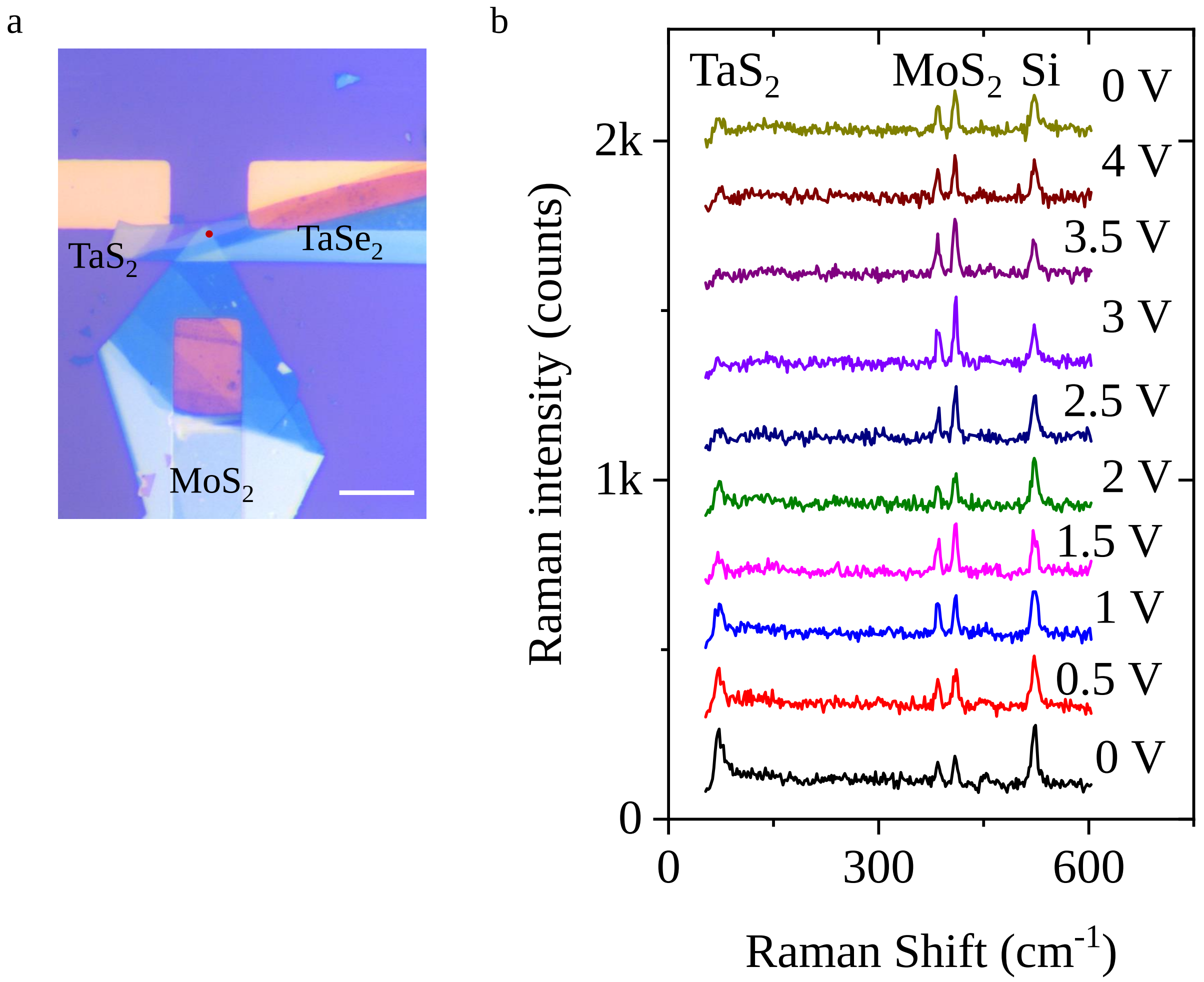


Figure 4: **Bias dependent Raman Spectra.** (a) Optical image of the fabricated $TaS_2/TaSe_2/MoS_2$ T-junction. Scale bar: 12 $\mu m$. (b) Bias dependent Raman intensity with light illumination of 532 nm at the junction region denoted by red dot in (a) depicting the absence of j-peaks thereby ruling out the $MoS_2$ phase transition from $2H$ to $1T$.

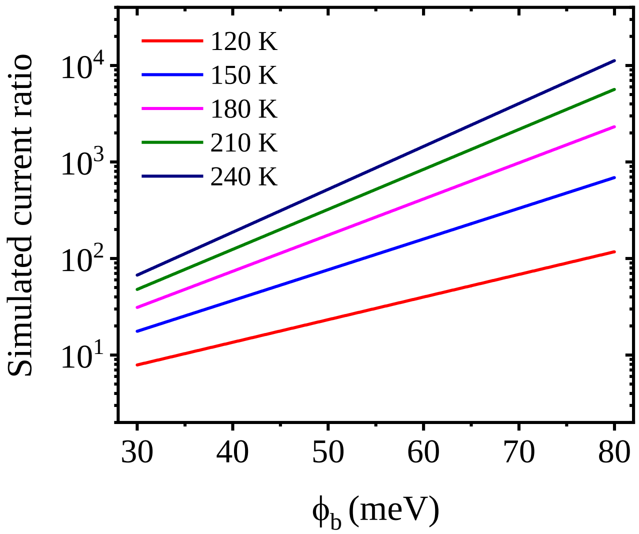


Figure 5: Simulated current ratio as a function of barrier height varying from 30 to 80 meV at 120 K, 150 K, 180 K, 210 K and 240 K with respect to 77 K using modified Richardson's equation.

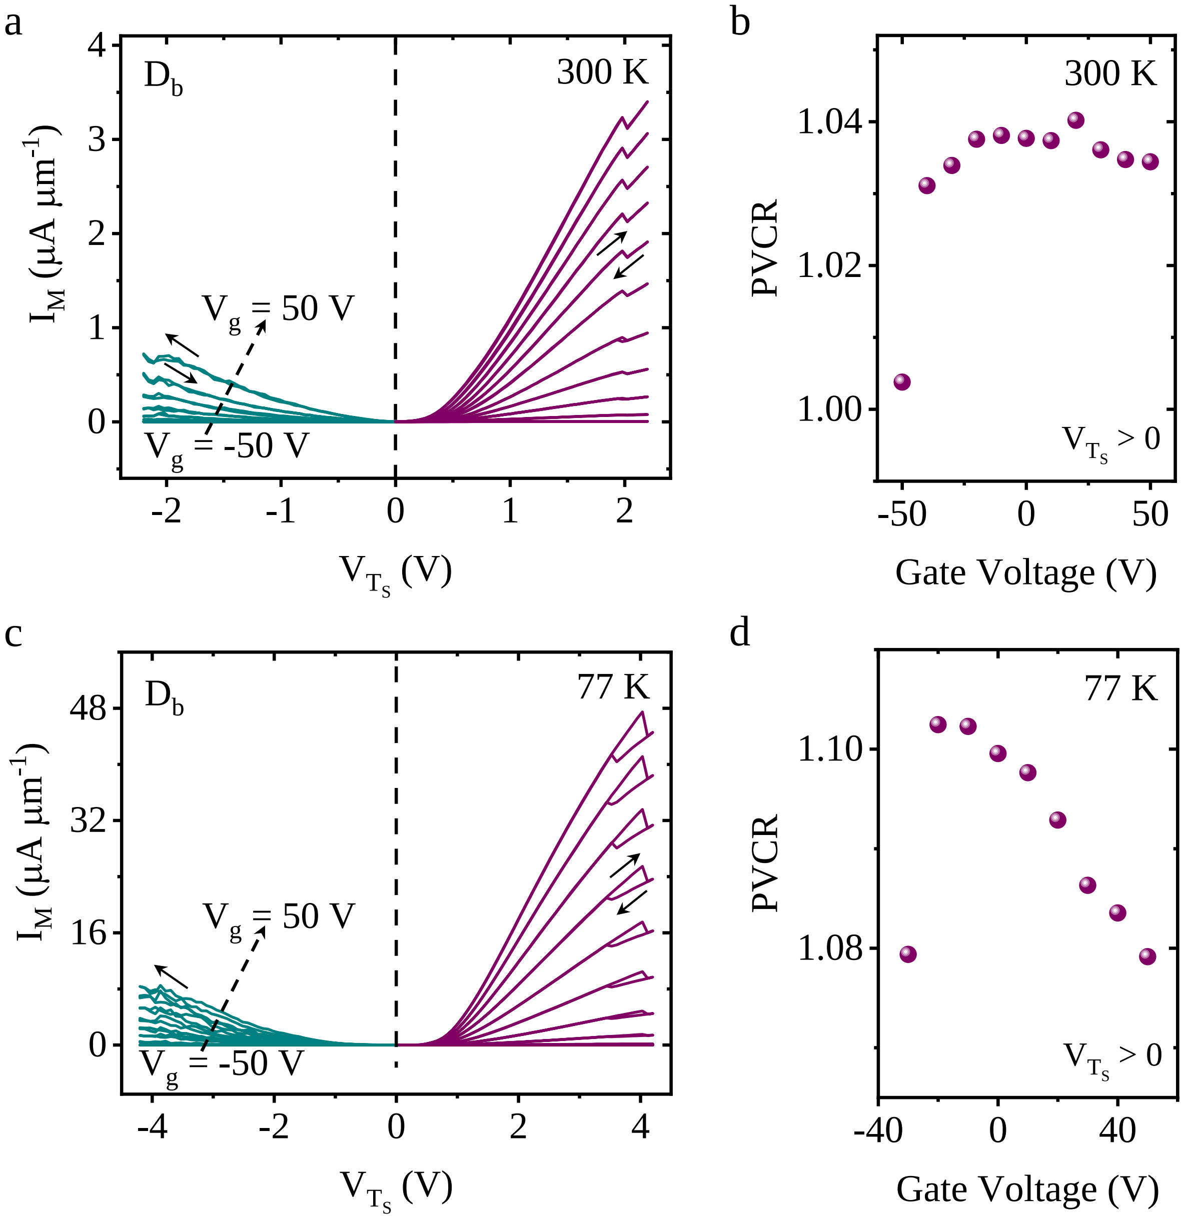


Figure 6: **Current decrement characteristics of device $\mathbf{D_b}$.** (a),(c) $I_M$ versus $V_{T_S}$ as the function of V$_g$ varying from −50 V to 50 V in steps of 10 V at 300 K [in (a)] and 77 K [in (c)]. Forward and reverse sweeps are indicated by black arrows. (b),(d) The corresponding PVCR values at 300 K [in (b)] and 77 K [in (d)] respectively.

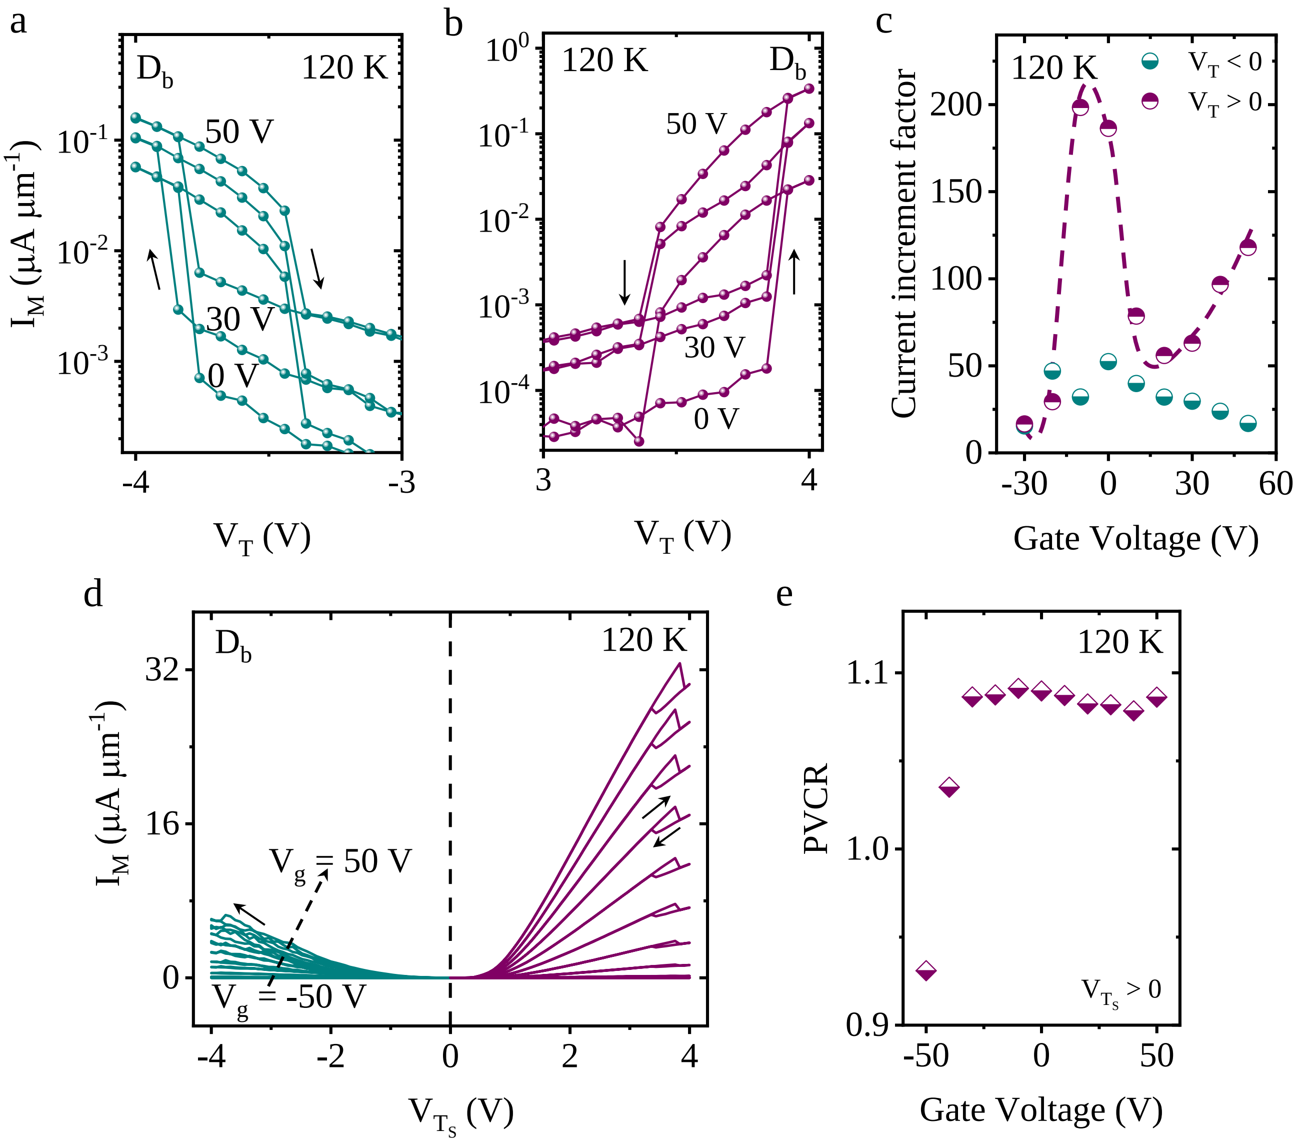


Figure 7: **Abrupt current increment and decrement characteristics of device $D_b$ at 120 K.** (a),(b) $I_M$ versus $V_T$ as the function of back gate voltage ($V_g$ = 0 V, 30 V and 50 V) showing abrupt current increment for $V_T < 0$ [in (a)] and $V_T > 0$ [in (b)] at 120 K. Forward and reverse sweeps are indicated by black arrows. (c) The extracted values of current increment factor for $V_T < 0$ and $V_T > 0$ at 120 K. (d) $I_M$ versus $V_{T_S}$ depicting current decrement for $V_g$ varying from −50 V to 50 V (Step size: 10 V) at 120 K. Forward and reverse sweeps are indicated by black arrows. (e) PVCR values extracted from (d).

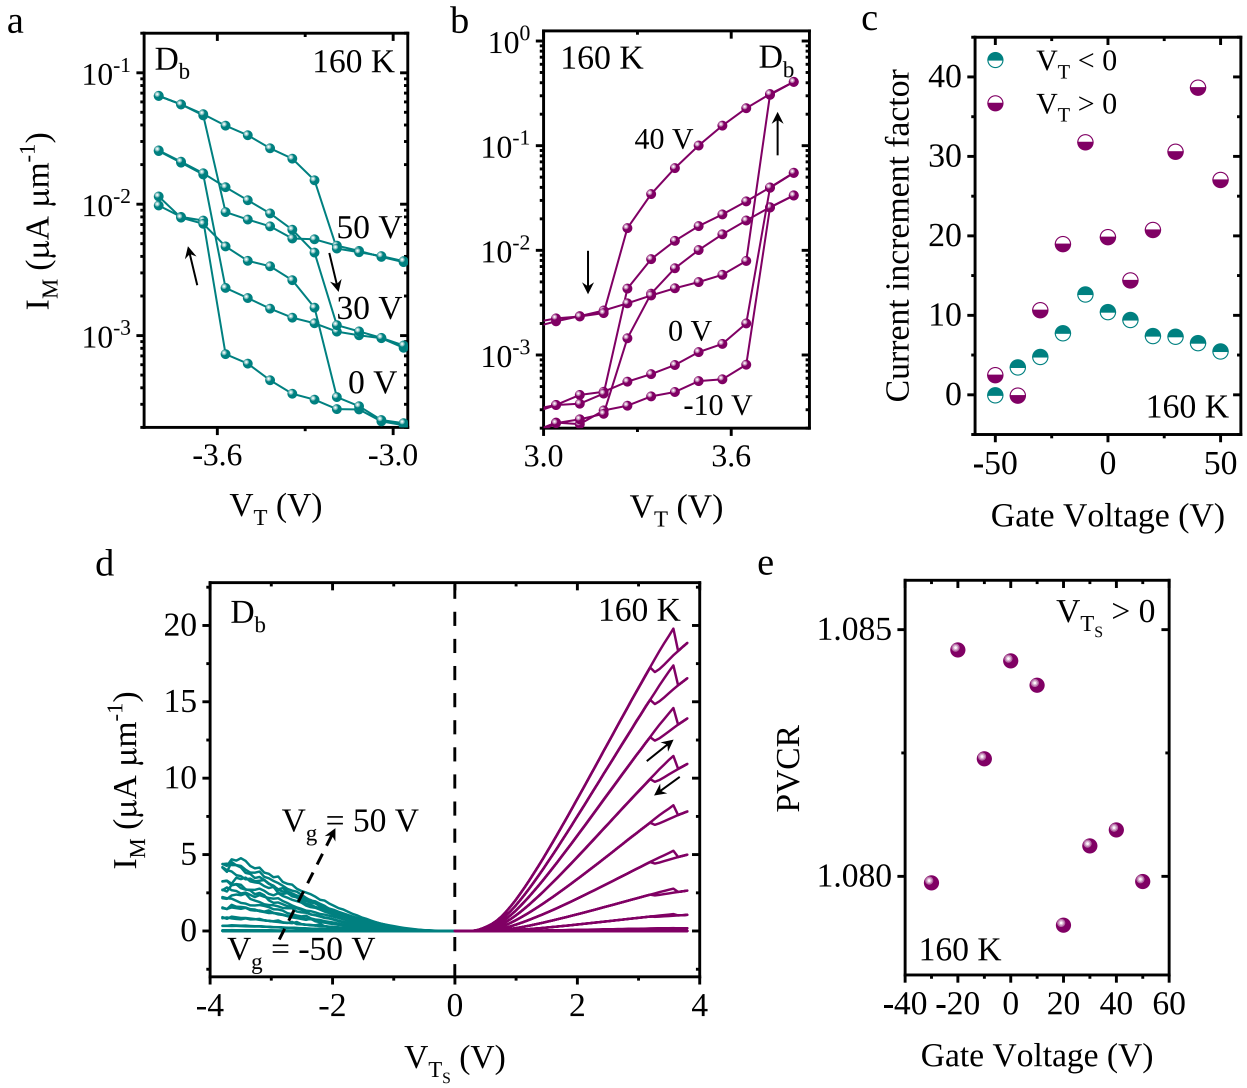


Figure 8: **Abrupt current increment and decrement characteristics of device $D_b$ at 160 K.** (a),(b) $I_M$ versus $V_T$ at different back gate voltage showing abrupt current increment for $V_T < 0$ [in (a)] and $V_T > 0$ [in (b)] at 160 K. Forward and reverse sweeps are indicated by black arrows. (c) The extracted values of current increment factor for $V_T < 0$ and $V_T > 0$ at 160 K. (d) $I_M$ versus $V_{T_S}$ depicting current decrement for $V_g$ varying from −50 V to 50 V (Step size: 10 V) at 160 K. Forward and reverse sweeps are indicated by black arrows. (e) PVCR values extracted from (d).

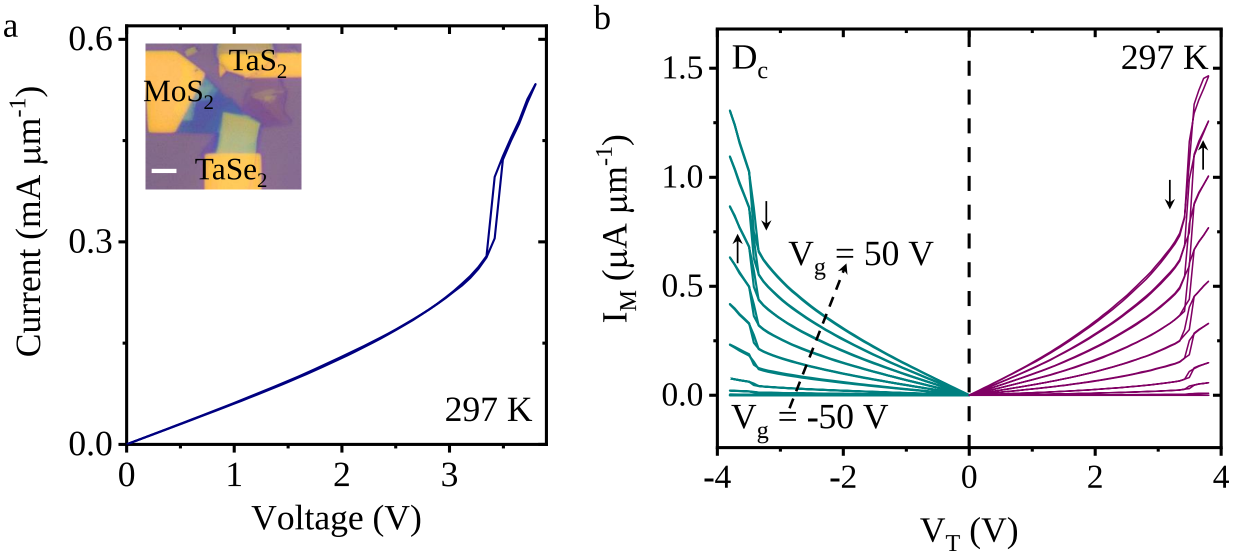


Figure 9: **Repeatability of device characteristics-I** (a) I-V characteristics of $TaS_2/TaSe_2$ junction of triple layered device $D_c$ showing joule heating induced current jump at 297 K. The inset shows the optical image of the fabricated device $D_c$. (b) $I_M$ versus $V_T$ as the function of $V_g$ varying from $-50$ V to 50 V in steps of 10 V at 297 K depicting abrupt current increment in $MoS_2$ current with maximum increment factor of about 1.55. Forward and reverse sweeps are indicated by black arrows.

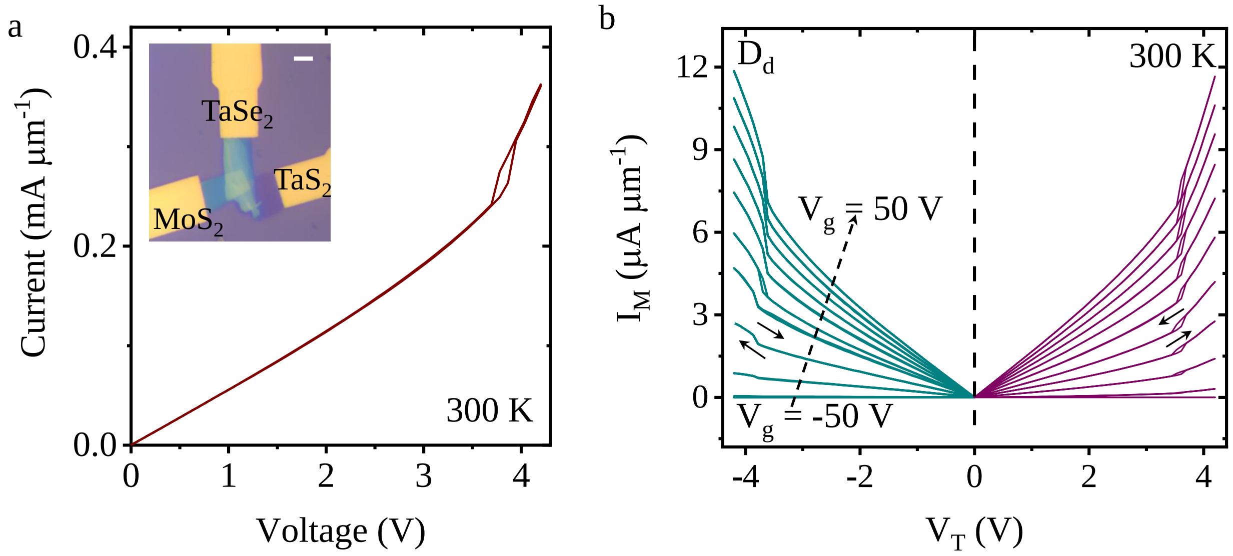


Figure 10: **Repeatability of device characteristics-II** (a) I-V characteristics of $TaS_2/TaSe_2$ junction of triple layered device $D_d$ showing joule heating induced current jump at 300 K. The inset shows the optical image of the fabricated device $D_c$. (b) $I_M$ versus $V_T$ as the function of $V_g$ varying from $-50$ V to 50 V in steps of 10 V at 300 K depicting abrupt current increment in $MoS_2$ current with maximum increment factor of about 2.35. Forward and reverse sweeps are indicated by black arrows.
